# Supplementary material for: Multispectral Video Fusion for Non-contact Monitoring of Respiratory Rate and Apnea
Source: arXiv:2004.09834 source file (2020-04-21)
Supplement: Supplementary file 1 [file ieeeTBME20_SM.pdf]

# Supplementary Material for "Multispectral Video Fusion for Non-contact Monitoring of Respiratory Rate and Apnea"

Gaetano Scebba, Giulia Da Poian, and Walter Karlen

G. Scebba, G. Da Poian and W. Karlen are with the Mobile Health Systems Lab, Institute of Robotics and Intelligent Systems, Department of Health Sciences and Technology, ETH Zurich, Switzerland (e-mails: gaetano.scebba@hest.ethz.ch, walter.karlen@ieee.org)

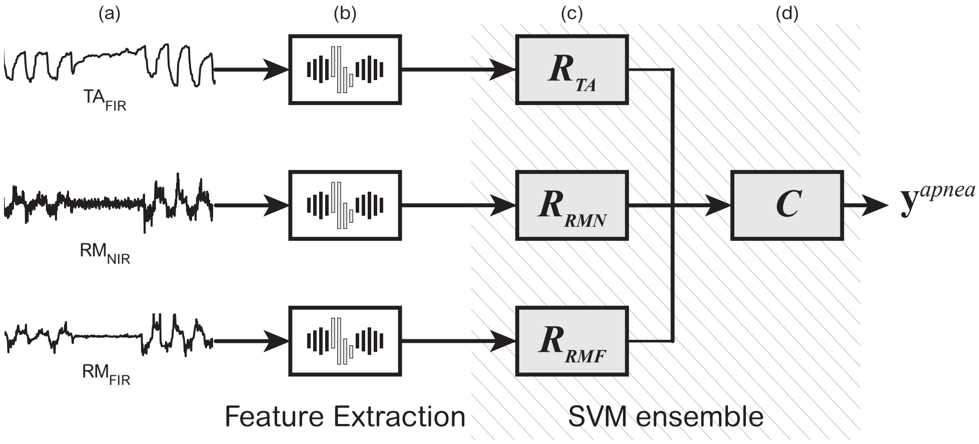


Fig. S1: Apnea detection model. (a) The respiratory signals $TA_{FIR}$, $RM_{NIR}$, and $RM_{FIR}$ are processed to extract (b) temporal and frequency domain features. (c-d) The SVM ensemble consists of one layer of support vector regression models $R_i$ and one support vector classification model C. (c) Each regression model $R_i$ computes the probability for the set of features extracted from the respiratory signal $i$ to belong to an apneic epoch. (d) The classification machine C aggregates the probabilities of the regression machines $R_i$ and computes the final output $y^{apnea}$

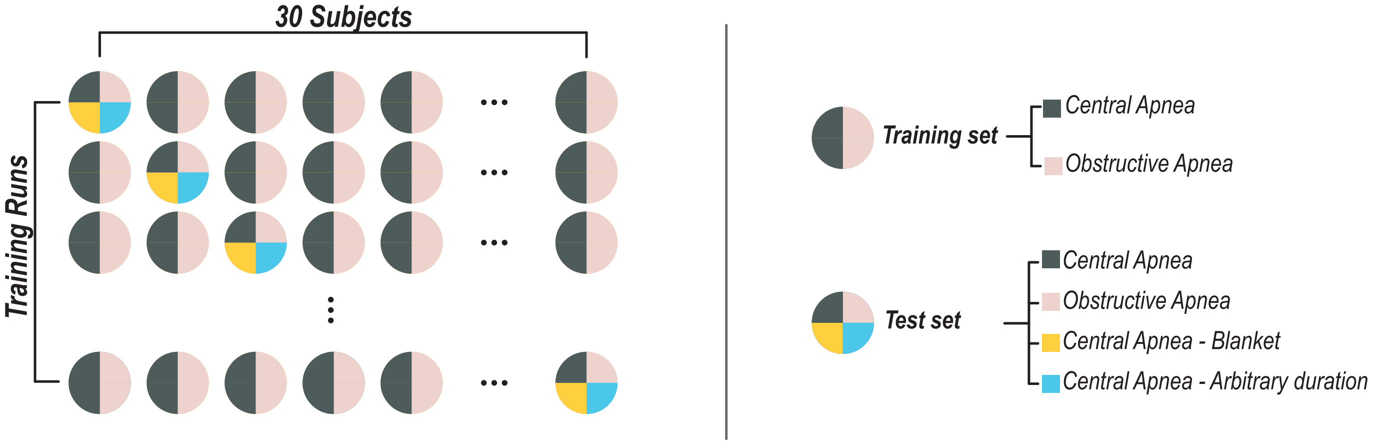


Fig. S2: Leave-one-subject-out evaluation scheme. At each run, the training and test sets included the data of 29 subjects and 1 subject respectively. The training set consisted of the recordings obtained from *Central Apnea* and *Obstructive Apnea* tasks, whereas the test set included the recordings obtained from all the tasks with apneic events.

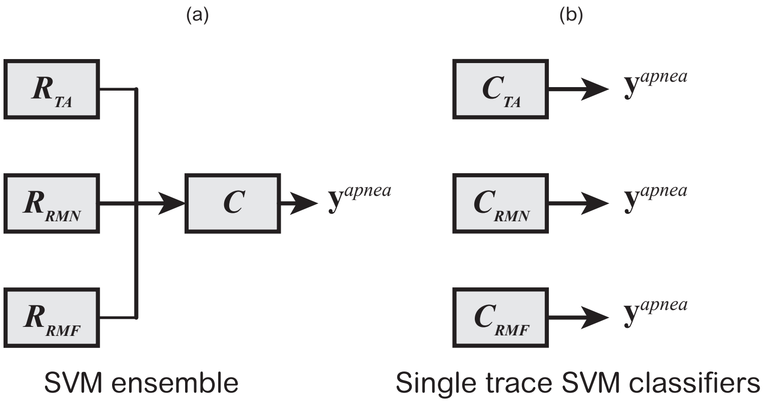


Fig. S3: Evaluation of the apnea detection performance. (a) The performance of the SVM ensemble to detect apnea were compared to the performance of three baseline SVN $C_i$. (b) Each classification machine was trained and tested using features extracted from the individual respiratory signals.

TABLE S1: Bias and limits of agreement from Bland-Altman analysis (lower is better), and Pearson correlation coefficient (higher is better) of the estimated RR using the signal quality based (SQb) Fusion and the median and mean fusion algorithms.

| Fusion Method | Bias (breaths/min) | Limits of agreement (breaths/min) | | $\rho$ |
|---|---|---|---|---|
| SQb Fusion | **0.46** | **-2.57** | **3.49** | **0.92** |
| Median | 0.92 | -3.32 | 5.16 | 0.84 |
| Mean | 0.94 | -3.81 | 5.69 | 0.79 |

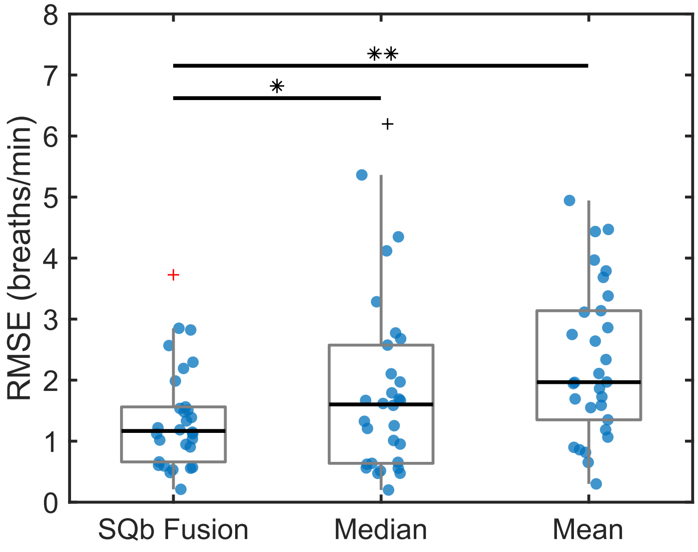


Fig. S4: Boxplot comparison of the root mean square error (RMSE) from the Spontaneous Breathing data for the signal quality based (SQb) Fusion, median and mean fusion algorithms (breaths/min). The boxplot represents the distribution across subjects. Bottom, middle, and top horizontal lines illustrate the lower quartile, median and upper quartile and crosses are outliers. Motion artifacts corrupted recording of subjects #22 (red cross). Asterisks indicate significant difference (* $p < 0.05$, ** $p < 0.01$).

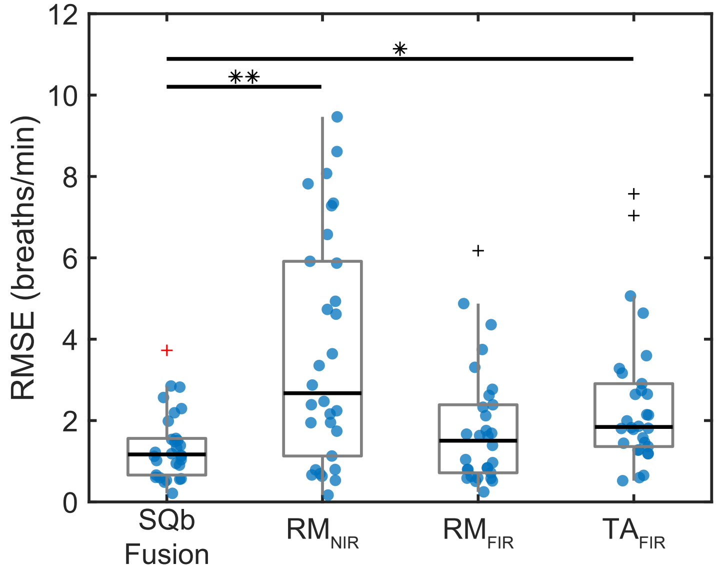


Fig. S5: Boxplot comparison of the root mean square error (RMSE) from the Spontaneous Breathing data for the signal quality based (SQb) Fusion algorithm and the algorithms based on the individual respiratory signals (breaths/min). The boxplot represents the distribution across subjects. Bottom, middle, and top horizontal lines illustrate the lower quartile, median and upper quartile, and crosses are outliers. Motion artifacts corrupted recording of subject #22 (red cross). Asterisks indicate significant difference (* $p < 0.05$, ** $p < 0.01$).
